# Supplementary material for: Understanding Robot Minds: Leveraging Machine Teaching for Transparent Human-Robot Collaboration Across Diverse Groups
Source: arXiv:2404.15472 source file (2024-04-23)
Supplement: Supplementary file 1 [file appendix.tex]

\section{Appendix}

\subsection{Human learner model for simulation}

% Rehprase - from HRI
Fig. \ref{fig:learner_model_evaluation} shows simulations of learner behavior for various categories of learners and different teaching frameworks. We evaluate the measure, probability of robot reward knowledge as the sum of weights of particles within the correct BEC area of the robot reward. The parameter values of $\beta, \, \delta\,\beta_c,\, \&\, \delta\,\beta_i$ were manually tuned to match the observed performance. By carefully choosing the parameters, the learner models can simulate close to the observed performance of actual human learners while seeing the same demonstrations and feedback. This demonstrates the model's applicability not only to model different types of learners but also for various teaching frameworks with different learning dynamics. Further, as seen in the top right of Fig. \ref{fig:learner_model_evaluation}, the learner is also to capture complicated learning behaviors that had trouble learning the first concept but performed very well after that.

\subsection{}
